# Supplementary material for: Thermal conductivity of the quantum spin liquid candidate EtMe3Sb[Pd(dmit)2]2: No evidence of mobile gapless excitations
Source: arXiv:1904.10402 source file (2019-09-20)
Supplement: Supplementary file 1 [file dmit131_SM_19sept2019_resub.pdf]

# Supporting Material

## X-Ray Diffraction Measurements

Single crystal X-ray diffraction (XRD) data on dmit-131 were collected by a Rigaku XtaLAB AFC11 (RCD3) system at RIKEN with monochromated Mo Kα radiation (Rigaku, Akishima-shi, Japan) at room temperature. Initial structures were solved and refined using SHELX within Olex2 [1], and then were refined on $F^2$ by the full-matrix least-squares method (SHELXT [2]). The ethyl group in the $EtMe_3Sb$ cation was treated by taking two equivalent positions around the two-fold axis.

In the Table S1 below we list all the samples investigated by XRD. The batch number of the crystal growth, the measured *R*-factor, and the orientation (where relevant) are indicated for all the samples. The *R*-factor, also known as discrepancy index, is a measure of the agreement between the crystallographic model and the actual XRD data. Low values indicate close agreement with the crystallographic model. Crystal data can be found in the attached CIF (crystallographic data format) files. For samples C1, D2, F1, G1, and Kyoto samples C and D, the XRD measurements were performed after the thermal conductivity measurements. Pristine samples are raw samples that have no contact and that were not otherwise measured. As can be seen from the list of R values in Table S1, all our samples have a similar crystalline quality to those measured by the Kyoto group. In particular, three samples from the very same batch, no. 752, all have similarly low *R*-factor: our sample G1, Yamashita's sample C and a pristine sample that has not been otherwise handled.

**Table S1:** List of the Sherbrooke and Kyoto dmit-131 samples measured by XRD at RIKEN, showing the sample reference, growth batch number, *R*-factor, and orientation.

| Sherbrooke dmit-131 samples | | | |
|---|---|---|---|
| Sample C1 | Batch No. 888 | *R*-factor = 2.20 % | a-axis |
| Sample D2 | Batch No. 1052 | *R*-factor = 3.95 % | a-axis |
| Sample F1 | Batch No. 751 | *R*-factor = 3.32 % | (see below) |
| Sample G1 | Batch No. 752 | *R*-factor = 2.23 % | a-axis |
| Pristine sample | Batch No. 888 | *R*-factor = 2.15 % | - |
| Pristine sample | Batch No. 1052 | *R*-factor = 2.42 % | - |
| Pristine sample | Batch No. 751 | *R*-factor = 3.32 % | - |

| Kyoto dmit-131 samples | | | |
|---|---|---|---|
| Sample C | Batch No. 752 | *R*-factor = 2.94 % | a-axis |
| Sample D | Batch No. 764 | *R*-factor = 3.43 % | a-axis |
| Pristine sample | Batch No. 752 | *R*-factor = 2.88 % | - |

In addition, synchrotron XRD measurements with a wide dynamic range were performed in order to clarify the differences in crystal imperfections and/or domain formations between Sherbrooke and Kyoto samples. The XRD measurements were conducted using a BL02B1 beam line equipped at the synchrotron facility SPring-8 in Japan. These experiments were performed at SPring-8 with the approval of the Japan Synchrotron Radiation Research Institute (JASRI) (Proposals No. 2019A0070).

The experimental conditions for the Spring-8 measurements are:
Wavelength: 0.562922 Å
Detector: CdTe PILATUS
Cooling: $N_2$-gas-blowing device
Temperature: 100 K (temp. slope: -3 K/min)

Using high-intensity synchrotron radiation at Spring-8, orientational ordering of the ethyl group in the cation $EtMe_3Sb^+$ at cryogenic temperatures can in principle be clarified by analyzing the domain formation. However, the ethyl group ordering and domain formation could not be determined precisely due to strong effects of the thermal vibrations even at 100K. It should be noted, however, that there was no significant difference in the pattern of thermal diffuse scattering at 100 K between our crystals and the Kyoto samples.

The measurements at SPring-8 also revealed that sample F1 is in fact made of two crystals with different in-plane orientations (Fig. S1). The above-mentioned crystal data for F1 (see Table S1) was obtained from one of them. Peak profiles of Bragg reflections measured at RIKEN show that both crystals making up F1 essentially have the same crystal quality (Fig. S2). Since there is very little planar transport anisotropy in dmit-131 (see Figs. 1a and 3 of main text), the adhesion of two crystals does not have any serious impacts on the in-plane thermal conductivity (see Table 1).

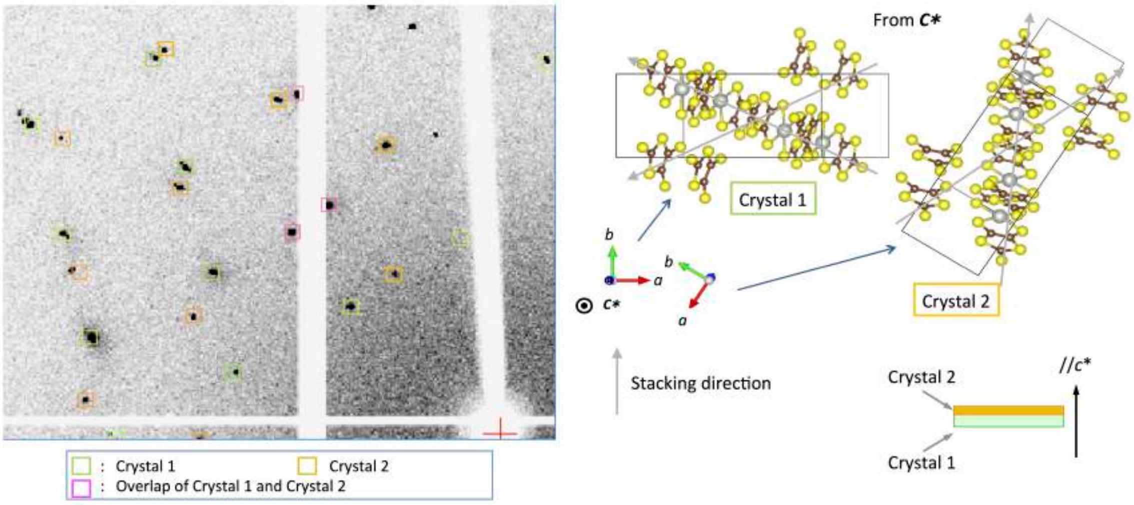


**Figure S1:** Bragg reflections from sample F1 (left) and orientations of two crystals (1 and 2) that form sample F1 (right)

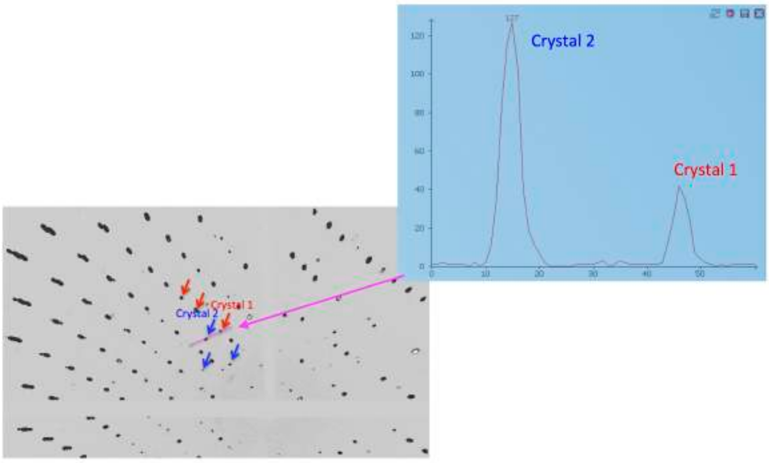


**Figure S2:** Peak profiles of Bragg reflections for sample F1 that consists of two crystals.

---

1 Dolomanov, O.V., Bourhis, L.J., Gildea, R.J, Howard, J.A.K. & Puschmann, H., *J. Appl. Cryst.* **42**, 339-341 (2009).

2 Sheldrick, G.M.. *Acta Cryst.* A**71**, 3-8 (2015).
